# Supplementary material for: LocoVLM: Grounding Vision and Language for Adapting Versatile Legged Locomotion Policies
Source: arXiv:2602.10399 source file (2026-02-11)
Supplement: Supplementary file 1 [file results_text_representation.tex]

\section{Effects of Text Representation on Retrieval Performance}\label{appendix:results_text_representation}
\begin{table*}[ht!]
    \centering
    \caption{Qualitative evaluation of retrieval performance using raw texts and preprocessed texts as images.}
    \label{table:retrieval}
    % chage table font size
    \footnotesize
    \begin{center}
    \resizebox{\linewidth}{!}{%
    \begin{tabular}{lm{0.18\linewidth}lm{0.18\linewidth}l}
    \hline

    \multicolumn{1}{c}{\multirow{2}{*}{\textbf{Query}}} 
    &\multicolumn{2}{c}{\textbf{Raw text}}
    &\multicolumn{2}{c}{\textbf{Text as image}} 
    \\ 

    &\multicolumn{1}{c}{\textbf{Retrieved instruction}} 
    &\multicolumn{1}{c}{\textbf{Parameters}}
    &\multicolumn{1}{c}{\textbf{Retrieved instruction}} 
    &\multicolumn{1}{c}{\textbf{Parameters}}\\
    \hline\hline

    \lang{you are a horse} 
    & \lang{jumping like a frog} 
    &\begin{tabular}[c]{@{}l@{}}
    $T=0.5$\\ 
    $\phi=[0,0,0,0]$\\ 
    $v^\text{limit}_x=0.7$\end{tabular}
    &\lang{run beautifully like a horse} 
    &\begin{tabular}[c]{@{}l@{}}
    $T=0.4$\\ 
    $\phi=[0.0,0.2,0.7,0.5]$\\ 
    $v^\text{limit}_x=1.5$\end{tabular}
    \\ \hline

    \lang{what is a horse?} 
    & \lang{a large puddle is in front of you, avoid it} 
    &\begin{tabular}[c]{@{}l@{}}
    $T=0.5$\\ 
    $\phi=[0.0,0.5,0.5,0.0]$\\ 
    $v^\text{limit}_x=0.5$\end{tabular}
    &\lang{run beautifully like a horse} 
    &\begin{tabular}[c]{@{}l@{}}
    $T=0.4$\\ 
    $\phi=[0.0,0.2,0.7,0.5]$\\ 
    $v^\text{limit}_x=1.5$\end{tabular}
    \\ \hline

    \lang{there's a bird} 
    & \lang{shh! someone is sleeping move quietly}  
    &\begin{tabular}[c]{@{}l@{}}
    $T=0.6$\\ 
    $\phi=[0.0,0.5,0.5,0.0]$\\ 
    $v^\text{limit}_x=0.3$\end{tabular}
    &\lang{let's hop like a rabbit!} 
    &\begin{tabular}[c]{@{}l@{}}
    $T=0.5$\\ 
    $\phi=[0.0,0.0,0.5,0.5]$\\ 
    $v^\text{limit}_x=0.8$\end{tabular}
    \\ \hline

    \lang{catch the bird!} 
    & \lang{shh! someone is sleeping move quietly}  
    &\begin{tabular}[c]{@{}l@{}}
    $T=0.6$\\ 
    $\phi=[0.0,0.5,0.5,0.0]$\\ 
    $v^\text{limit}_x=0.3$\end{tabular}
    &\lang{crawl low to the ground like a lion stalking prey}
    &\begin{tabular}[c]{@{}l@{}}
    $T=0.6$\\ 
    $\phi=[0.0,0.5,0.0,0.5]$\\ 
    $v^\text{limit}_x=0.2$\end{tabular}
    \\ \hline

    \lang{run! there's a danger!} 
    & \lang{there's an icy patch! go carefully!}  
    &\begin{tabular}[c]{@{}l@{}}
    $T=0.7$\\ 
    $\phi=[0.0, 0.5, 0.5, 0.0]$\\ 
    $v^\text{limit}_x=0.4$\end{tabular}
    &\lang{there's a predator behind you, move fast!} 
    &\begin{tabular}[c]{@{}l@{}}
    $T=0.7$\\ 
    $\phi=[0.0, 0.2, 0.7, 0.5]$\\ 
    $v^\text{limit}_x=1.5$\end{tabular}
    \\ \hline
    
    \end{tabular}
    }
    \end{center}
\end{table*}

We further evaluate how retrieval performance changes when the text query is represented as a text image. Table~\ref{table:retrieval_accuracy} shows that retrieval performance improves when the text query is represented as a text image, with an overall improvement of approximately $15$ out of $100$ instructions. This finding suggests that the VLM is more effective at understanding text queries when the text is represented as an image, because the VLM was primarily trained on image-text pairs.

To qualitatively evaluate these results, we sampled several retrieval examples summarized in Table~\ref{table:retrieval}. Out of five examples, the VLM tends to retrieve irrelevant instructions when given with text queries, such as \lang{jumping like a frog} for the query \lang{you are a horse}. However, when the text query is represented as a text image, the VLM retrieves more relevant instructions, such as \lang{run beautifully like a horse} for the same query. 

The reflection from this result is that pre-trained VLMs, such as CLIP~\cite{radford2021learning}, BLIP~\cite{li2023blip}, and BLIP-2~\cite{Hunter:2007}, were primarily trained using contrastive learning on image-text pairs. Consequently, they are more proficient at understanding text queries when represented as images.
