# Supplementary material for: LocoVLM: Grounding Vision and Language for Adapting Versatile Legged Locomotion Policies
Source: arXiv:2602.10399 source file (2026-02-11)
Supplement: Supplementary file 2 [file results_gait_tracking.tex]

\section{Compliant Gait Tracking Performance}\label{appendix:results_gait_tracking}
\input{\MainPath/experiments/tables/gait_tracking}
We evaluated the gait tracking performance with different compliance thresholds~$\delta$ to assess the trade-off between accuracy and robustness in the proposed compliant contact tracking method. Table~\ref{table:gait_tracking} summarizes the results obtained from simulation using $1,\!000$ rollouts and four different values of $\delta$.
