# Supplementary material for: LocoVLM: Grounding Vision and Language for Adapting Versatile Legged Locomotion Policies
Source: arXiv:2602.10399 source file (2026-02-11)
Supplement: Supplementary file 3 [file results_interpretation.tex]

\section{LocoVLM Interpretation of Queries Out of the Database}\label{appendix:results_interpretation}
Table~\ref{table:outofdb_queries} shows the capability of \acro on providing meaningful interpretations for queries that are not present in the database. 
\begin{table}
    \vspace{-15pt}
    \centering
    % chage table font size
    \scriptsize

    \caption{VLM interpretations for queries that are not present in the skill database.}
    \label{table:outofdb_queries}
    \begin{center}
    \begin{tabular}{m{0.4\linewidth}m{0.48\linewidth}}
    
    \hline
    \multicolumn{1}{c}{\textbf{Query}} & \multicolumn{1}{c}{\textbf{Interpretation}} \\
    \hline\hline

    \lang{you are a kangaroo} & \lang{let's jump like a rabbit} \\ \hline
    \lang{the road is slippery} & \lang{the floor is wet, walk cautiously} \\ \hline
    \lang{how does a frog jump?} & \lang{show me some pronk} \\ \hline
    \lang{this is a library!} & \lang{shh! Someone is sleeping, move quietly} \\ \hline
    
    \end{tabular}
    \end{center}
    \vspace{-15pt}
\end{table}
